# Supplementary material for: Risk-Averse Certification of Bayesian Neural Networks
Source: arXiv:2411.19729 source file (2024-11-29)
Supplement: Supplementary file 1 [file Appendix.tex]

% \section*{Appendix}
% \begin{lemma}\label{Eq:LCWd}
% Suppose that the function $h:\Rb^n \mapsto \Rb$ is Lipschitz continuous with respect to a constant $L\geq 0$. For any two probability distribution $\Prob{Y}, \Prob{Y}' \in \mathcal{P}(\mathbb{Y})$, 
% \begin{align}
%     | \int_{\mathbb{Y}} h(\xi)\Prob{Y}(d \xi)-  \int_{\mathbb{Y}} h(\xi) \Prob{Y}'(d \xi)| \leq L d^{\mathbb{Y}}_{\text W}(\Prob{Y},\Prob{Y}'). 
% \end{align}
% \end{lemma}
% \subsection*{Proof of Theorem 2 \zf{We probably do not present Theorem 2. Then this section along with Lemma 7 needs to be removed}}
%     Recall that $Perf= \int_{\mathbb{Y}}  h(\xi) \Prob{Y}(d\xi)$. We have that 
% \begin{align}\label{eq:thm2:1}
%    & | \int_{\mathbb{Y}} h(\xi)\Prob{Y}(d \xi)-  \int_{\hat{\mathbb{Y}}_N} h(\xi)\bar{\Prob{Y}}(d \xi)| \nonumber\\
%    =&| \int_{\mathbb{Y}} h(\xi)\Prob{Y}(d \xi)- \int_{\hat{\mathbb{Y}}_N} h(\xi)\Prob{Y}(d \xi) \nonumber  \\
%    & +\int_{\hat{\mathbb{Y}}_N} h(\xi)\Prob{Y}(d \xi) -\int_{\hat{\mathbb{Y}}_N} h(\xi)\empProb{Y}{N}(d \xi) \nonumber \\ 
%    & +\int_{\hat{\mathbb{Y}}_N} h(\xi)\empProb{Y}{N}(d \xi)-\int_{\hat{\mathbb{Y}}_N} h(\xi)\bar{\Prob{Y}}(d \xi)| \nonumber \\
%    \leq  &| \int_{\mathbb{Y}} h(\xi)\Prob{Y}(d \xi)- \int_{\hat{\mathbb{Y}}_N} h(\xi)\Prob{Y}(d \xi)| \nonumber  \\
%    & +|\int_{\hat{\mathbb{Y}}_N} h(\xi)\Prob{Y}(d \xi) -\int_{\hat{\mathbb{Y}}_N} h(\xi)\empProb{Y}{N}(d \xi)| \nonumber \\ 
%    & +|\int_{\hat{\mathbb{Y}}_N} h(\xi)\empProb{Y}{N}(d \xi)-\int_{\hat{\mathbb{Y}}_N} h(\xi)\bar{\Prob{Y}}(d \xi)|.
% \end{align}  

% For the first item, it follows from the boundedness of $h(y)$ over $\mathbb{Y}$ and   Proposition~\ref{Prop: risk bound} that   with probability no less than $1-\beta_1$, 
% \begin{align} \label{eq:thm2:2}
% | \int_{\mathbb{Y}} h(\xi)\Prob{Y}(d \xi)- \int_{\hat{\mathbb{Y}}_N} h(\xi)\Prob{Y}(d \xi)| \leq h_{\max} \epsilon_1. 
% \end{align}  

% Let us address the second item. 
% According to Lemma~\ref{Eq:LCWd},  Proposition~\ref{Pro:evadis}, and  \eqref{eq:thm2:2}, it follows that   with probability no less than $1-\max\{\beta_1,\beta_2\}$,   
% \begin{align}  \label{eq:thm2:3}
% &|\int_{\hat{\mathbb{Y}}_N} h(\xi)\Prob{Y}(d \xi) -\int_{\hat{\mathbb{Y}}_N} h(\xi)\empProb{Y}{N}(d \xi)| \nonumber \\
% =({\color{red}\leq?})& |\int_{ \mathbb{Y}} h(\xi)\Prob{Y}(d \xi)  -\int_{\mathbb{Y}} h(\xi)\empProb{Y}{N}(d \xi)-\int_{\hat{\mathbb{Y}\setminus (\mathbb{Y}}_N \cap \mathbb{Y})} h(\xi)\Prob{Y}(d \xi)|  \nonumber \\
% \leq & |\int_{ \mathbb{Y}} h(\xi)\Prob{Y}(d \xi)  -\int_{\mathbb{Y}} h(\xi)\empProb{Y}{N}(d \xi)|+|\int_{\hat{\mathbb{Y}\setminus (\mathbb{Y}}_N \cap \mathbb{Y})} h(\xi)\Prob{Y}(d \xi)| \nonumber \\
% \leq & L \epsilon_2 +  h_{\max} \epsilon_1.  
% \end{align} 

% Similarly, we can address the third item by concluding that with probability no less than $1-\beta_2$,  
% \begin{align}  \label{eq:thm2:4}
% |\int_{\hat{\mathbb{Y}}_N} h(\xi)\empProb{Y}{N}(d \xi)-\int_{\hat{\mathbb{Y}}_N} h(\xi)\bar{\Prob{Y}}(d \xi)|  \leq L \epsilon_3.
% \end{align}  
% Combining \eqref{eq:thm2:1}--\eqref{eq:thm2:4}, we have
% \begin{align}
%    & | \int_{\mathbb{Y}} h(\xi)\Prob{Y}(d \xi)-  \int_{\hat{\mathbb{Y}}_N} h(\xi)\bar{\Prob{Y}}(d \xi)| \nonumber \\
%    \leq & 2 h_{\max} \epsilon_1 +L \epsilon_2+L \epsilon_3 :=\zeta.
% \end{align}  
% % Thus, we conclude that 
% % Following Propositions~\ref{Prop: risk bound}--\ref{Pro:evadis}, 
% Thus, we have that with probability no less than $1-\max\{\beta_1,\beta_2\}$, 
% \begin{align}
%      Perf &\leq \int_{\hat{\mathbb{Y}}_N} h(\xi)\bar{\Prob{Y}}(d \xi) + \zeta \nonumber \\
%      &\leq \sup_{\Prob{Y}'\in \mathbb{B}_{\epsilon_3}(\empProb{Y}{N})}\int_{\hat{\mathbb{Y}}_N} h(\xi)\Prob{Y}'(d \xi) + \zeta,
% \end{align}
% % and {\color{red}
% % \begin{align}
% %      Perf &\geq \int_{\hat{\mathbb{Y}}_N} h(\xi)\bar{\Prob{Y}}(d \xi) - \zeta \nonumber \\
% %      &\geq \inf_{\Prob{Y}'\in \mathbb{B}_{\epsilon_3}(\empProb{Y}{N})}\int_{\hat{\mathbb{Y}}_N} h(\xi)\Prob{Y}'(d \xi) - \zeta,
% % \end{align}}
% where the ambiguity set $\mathbb{B}_{\epsilon_3}(\empProb{Y}{N})=\{\Prob{Y}' \mid d^{\hat{\mathbb{Y}}_N}_{\text W}(\Prob{Y}',\empProb{Y}{N})\leq \epsilon_3 \}$. 
%\begin{proof}
 %   \begin{eqnarray}  
%		| \int_ {\mathbb{S} \cap\mathbb{Y}}{\text Pr}^y(dy)-  \int_ {\mathbb{S} \cap\hat{\mathbb{Y}}}\bar{\text Pr}^y(dy)| \leq \underbrace{\epsilon_1 + 2\epsilon_2}_{:=\zeta}.
%	\end{eqnarray}  
%\end{proof}


% \textcolor{blue}{
% Strong duality: \cite{esfahani2015data}
% \begin{align}
%     &\sup_{\Prob{Y}'\in \mathbb{B}_{\epsilon_3}(\empProb{Y}{N})}\int_{\hat{\mathbb{Y}}_N} h(\xi)\Prob{Y}'(d \xi) \nonumber \\
%     &= \inf_{\beta\geq 0}\{ \frac{1}{N} \sum_{i=1}^N \max_{\xi \in \empProb{Y}{N}} \{ h(\xi) -\beta \| \xi - y_i\|  \} + \epsilon_3 \beta \}
% \end{align}
% According to \cite{esfahani2015data}, the worst case distribution is characterized by 
% $$
% Q^* = \frac{1}{N}\sum_{i=1}^N \delta_{\xi_{i}^*} \; with \; \xi_i^*: = \hat{\xi}_i - q_i^*,
% $$
% where $q_i^*$ is the value of $q_i$ that attains the supremum of the following finite convex program
% \begin{align}
%     \sup_{q_i} \quad  &\frac{1}{N}\sum_{i=1}^N l(\hat{\xi}_i - q_i) \nonumber \\
%     s.t. \quad & \frac{1}{N} \sum_{i=1}^N \left\| q_i\right\| \leq \epsilon_3 \nonumber \\
%     &\hat{\xi}_i -q_i \in  \hat{\mathbb{Y}}_N, \forall i \leq N.
% \end{align}
% Then, 
% \begin{align}
%     \sup_{\Prob{Y}'\in \mathbb{B}_{\epsilon_3}(\empProb{Y}{N})}\int_{\hat{\mathbb{Y}}_N} h(\xi)\Prob{Y}'(d \xi) = \mathbb{E}_{Q_*}[h(\xi)] = \frac{1}{N}\sum_{i=1}^N l(\xi_i^*).
% \end{align}}


% \noindent \textbf{Proof of Proposition 3:}
% Define 
% \begin{equation}
% \tilde{\Prob{Y}}(y)=\begin{cases}
% 	\frac{1}{1-\gamma}\Prob{Y}(y), \text{ if } y\in \mathbb{Y}\cap \hat{\mathbb{Y}}_N, \\
% 	0,  \text{ if } y \in \hat{\mathbb{Y}}_N \backslash ( \mathbb{Y}\cap \hat{\mathbb{Y}}_N ),
% \end{cases}
% \end{equation}
% where $\gamma = \nu(\mathbb{Y}\cap \hat{\mathbb{Y}}_N )$. According to Proposition 1, we have $\gamma \leq \epsilon_1$ with probability at least $1-\beta_1$. 
% Define 
% \begin{equation}
% \nu_0(y)=\begin{cases}
% 	0, \text{ if } y\in \mathbb{Y}\cap \hat{\mathbb{Y}}_N, \\
% 	\frac{1}{\gamma}\bar{\nu}(y), \text{ if } y \in \hat{\mathbb{Y}}_N \backslash ( \mathbb{Y}\cap \hat{\mathbb{Y}}_N ),
% \end{cases}
% \end{equation}
% We have $\bar{\nu} = (1-\gamma) \tilde{\nu} + \gamma \nu_0$ and $\tilde{\nu}$ and $\nu_0$ are mutually singular. Then,
% \begin{align}\label{eq:p2:1}
%     &d^{\hat{\mathbb{Y}}_N}_{\text W}(\bar{\Prob{Y}},\empProb{Y}{N}) = d^{\hat{\mathbb{Y}}_N}_{\text W}( (1-\gamma) \tilde{\nu}+ \gamma \nu_0,\empProb{Y}{N}) \nonumber \\
%     \leq & (1-\gamma) d^{\hat{\mathbb{Y}}_N}_{\text W}( \tilde{\nu},\empProb{Y}{N}) + \gamma d^{\hat{\mathbb{Y}}_N}_{\text W}(\nu_0,\empProb{Y}{N}),
% \end{align}
% where the last inequality follows from the convexity of Wasserstein distance.
% Denote by $\rho( \hat{\mathbb{Y}}_N)$ the diameter of the support of $\hat{\mathbb{Y}}_N$.
% Then, we have
% \begin{align}\label{eq:p2:2}
%     \gamma d^{\hat{\mathbb{Y}}_N}_{\text W}(\nu_0,\empProb{Y}{N}) \leq \gamma \rho( \hat{\mathbb{Y}}_N) \leq \epsilon_1 \rho( \hat{\mathbb{Y}}_N)
% \end{align}
% with probability at least $1-\beta_1$.
% Since both $\tilde{\nu}$ and $\hat{\nu}_N$ have measure $0$ outside $ \mathbb{Y}\cap \hat{\mathbb{Y}}_N$, we have
% \begin{align}\label{eq:p2:3}
%     &d^{\hat{\mathbb{Y}}_N}_{\text W}( \tilde{\nu},\empProb{Y}{N})
%     = d^{\mathbb{Y}}_{\text W}( \tilde{\nu},\empProb{Y}{N}) \nonumber \\
%     \leq &d^{\mathbb{Y}}_{\text W}( \tilde{\nu}, \nu) + d^{\mathbb{Y}}_{\text W}( \nu, \empProb{Y}{N}) \nonumber \\
%     \leq & \frac{\gamma}{1-\gamma} \rho(\mathbb{Y}) + d^{\mathbb{Y}}_{\text W}( \nu, \empProb{Y}{N}) \nonumber \\
%     \leq & \frac{\epsilon_1}{1-\epsilon_1} \rho(\mathbb{Y}) + \epsilon_2,
% \end{align}
% with probability no less than $1-\beta_1 - \beta_2$.
% The first inequality follows from the triangle inequality of Wasserstein distance. The second inequality follows when the transportation plan is selected as transporting $\frac{\gamma}{1-\gamma}$ fraction of $\tilde{\nu}$ to that of $\nu$ supported on $\mathbb{Y} \backslash ( \mathbb{Y}\cap \hat{\mathbb{Y}}_N)$.
% Define the events $A = \{ \gamma > \epsilon_1\}$ and $B=\{ d^{\mathbb{Y}}_{\text W}(\Prob{Y},\empProb{Y}{N})\geq \epsilon_2\}$. The last inequality holds with probability at least $1-\beta_1 -\beta_2$ since $1- \mathbb{P}( A \cup B ) \geq 1 - \mathbb{P}(A) - \mathbb{P}(B) \geq 1-\beta_1 -\beta_2$.

% Combining \eqref{eq:p2:1}--\eqref{eq:p2:3}, we have
% \begin{align}
%      d^{\hat{\mathbb{Y}}_N}_{\text W}(\bar{\Prob{Y}},\empProb{Y}{N}) 
%     \leq & \frac{\epsilon_1}{1-\epsilon_1} \rho( \hat{\mathbb{Y}}_N) + \epsilon_1 \rho(\mathbb{Y}) + \epsilon_2.
% \end{align}
% The proof is complete.
